# Supplementary material for: Image based Eye Gaze Tracking and its Applications
Source: arXiv:1907.04325 source file (2019-07-09)
Supplement: Supplementary file 1 [file AppendixII.tex]

\chapter{LK-MOSSE Tracker}{LK-MOSSE Tracker}
%\graphicspath{{Chapter5_eac/pics/}}

\section{Introduction}
Face detection is an important stage in many computer vision applications like face recognition, facial expression analysis and gaze tracking. Several methods has been proposed  \cite{viola2001rapid,rowley1998neural,yang1994human,yang1996real,yang2000face,yow1997feature,zhu2000fast,jones2001rapid,rowley1998neural,ben2006fuzzy,han2000fast,hjelmaas2001face,kong2007multi,hsu2002face} in literature for face detection. Among these methods, the use of Haar-like features \cite{viola2001rapid,jones2001rapid,hjelmaas2001face,kong2007multi,hsu2002face} is found to be quite robust. The direct application of Viola-Jones approach has certain disadvantages such as 1) Comutational overload while using for realtime applications , 2) detects only frontal faces and 3) No tracking for video sequences. We have used a simple but effective approach for solving these issues.
\section{The Algorithm}
\textbf{Haar-like Features}\\
Haar-like features \cite{viola2001rapid,jones2001rapid} are certain features used in image processing, they are similar to Haar wavelets. An algorithm for face detection using Haar-like features was first developed by Viola et. al. \cite{viola2001rapid,jones2001rapid} and was later extended by Lienhart et. al.\cite{lienhart2002extended}. The implementation of algorithm was fast since the features could be computed easily once the integral image is computed. The algorithm uses a cascade of classifiers to identify the face location.  We have made three additions to make it suitable for our real-time applications. We assume that the field of view of the camera contains a face, and the location of face does not change abruptly.
Based on these assumptions we use a tracking framework using Kalman Filter (KF) to constrain the area of search. The three modifications are discussed below.
\subsection{Speeding up operation with downsampling and ROI remapping }
In the original algorithm, the input image at full resolution is used for face detection. Integral images \cite{viola2001rapid} are computed from the full resolution images. Once the integral images are computed, any one of these Haar-like features can be obtained at any scale or location in constant time. The classifier then searches over multiple scales in a sliding window fashion. To speedup the detection, the size of the image as well as the size of the face to be searched can e limited. Here we assume that the face is close to the camera (maximum 1 meter from the camera), based on this contraint we downsample the image by a scale factor of four. This limits the number of steps for face size as well as the spatial area for search which reduces the computational time considerably. Eventhough face detection is carried ut in the downsampled image, the detected ROI is remapped to the original image which reatains high resolution images for further applications like face recognition or eye detection. A schematic of the remapping sche is shown in the figure.
It was emprically obeserved that the accuracy of face detection was not affected much with scale factors upto four (as long as face was near to the camera).

\begin{figure}[h]
\begin{center}
   \includegraphics[width=1\linewidth]{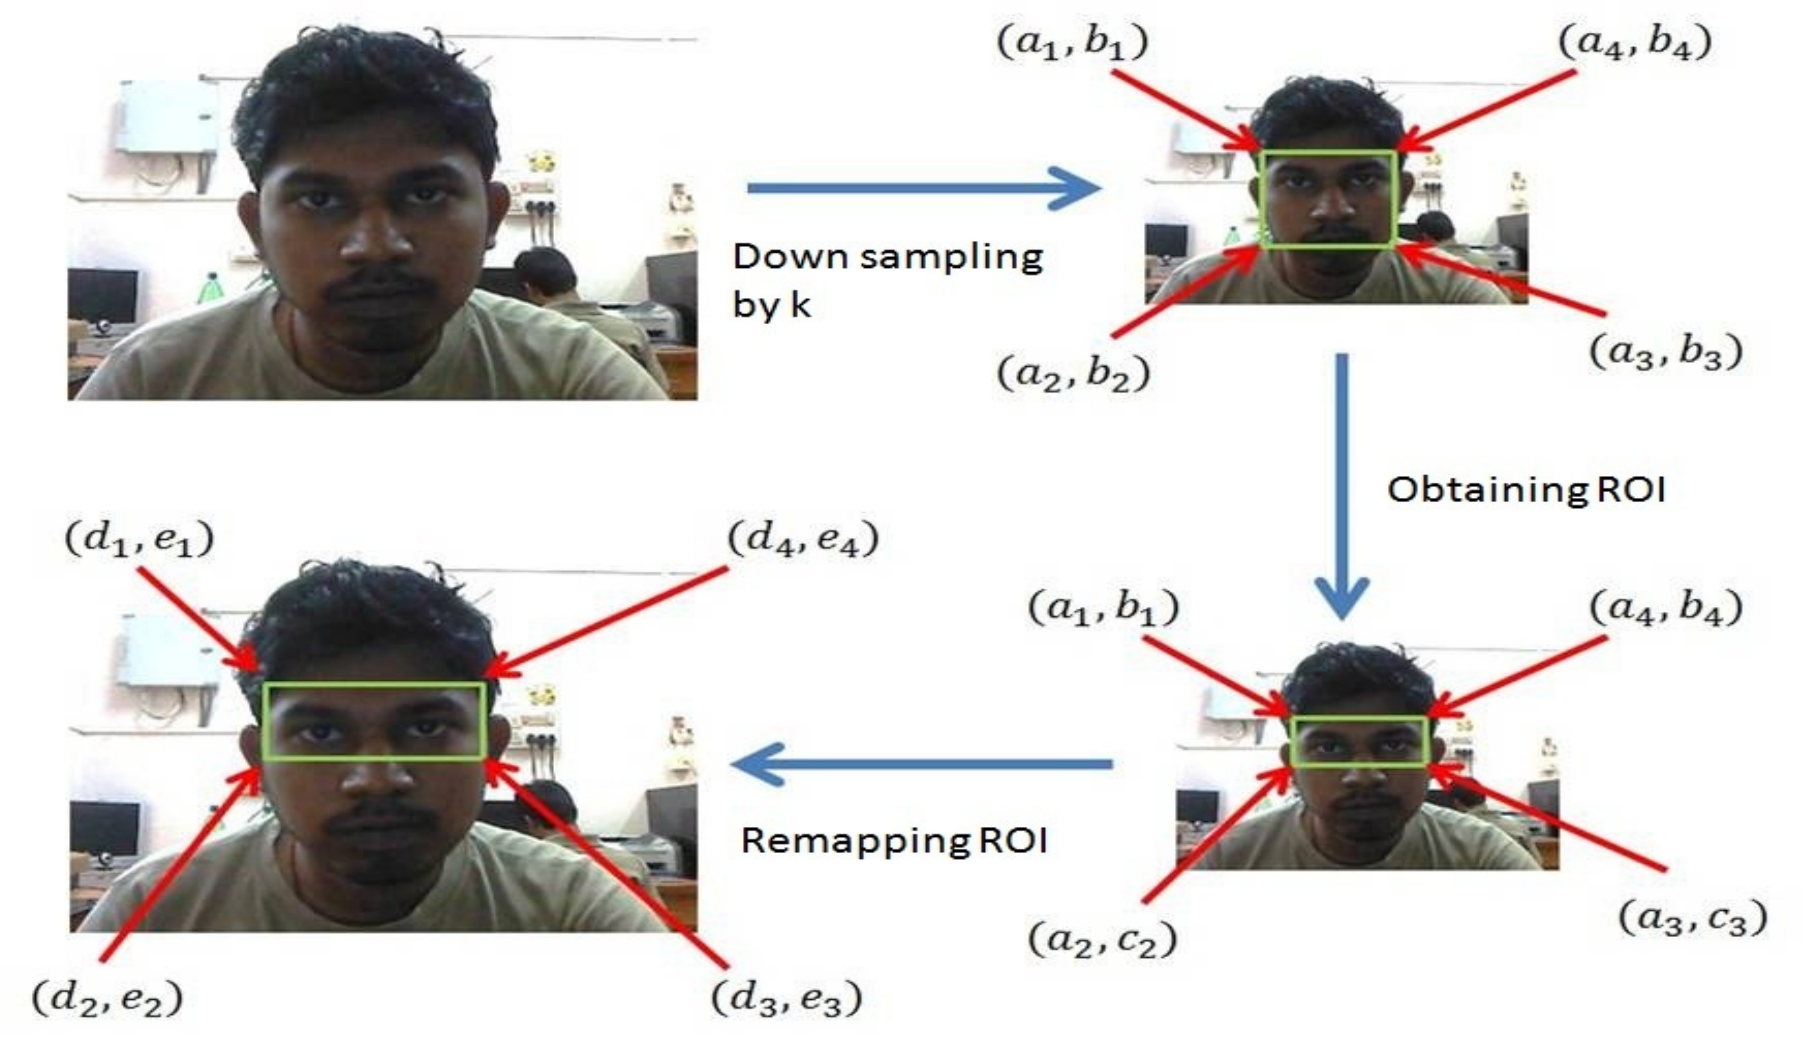}
\end{center}
   \caption{ROI remapping}
\label{fig:roi_remap}
\end{figure}

\subsection{Tilted face detection using an affine tranformation}
Direct application of Viola-Jones algorithm detects frontal upright images only.  Face detection along with subsequent stages fail if there is a moderate amount of tilt.  Most of the applications require he detection of faces in tilted conditions as well. An affine transformation based method is adopted for the detection of tilted (in plane rotated) faces. The rotation matrix can be found for an “n” dimensional image once its size, center and angle of rotation needed are known. This is added along with down sampling to make a robust face detection algorithm. The algorithm starts with applying the affine trasformation based on the face detection result from the previous frame. Fig. \ref{fig:tilted_face} shows tilted face detection using an affine transformation. A detailed description of this algorithm is provided in our earlier works \cite{dasgupta2013board,dasgupta2013vision}. 
\begin{figure}[h]
\begin{center}
   \includegraphics[width=1\linewidth]{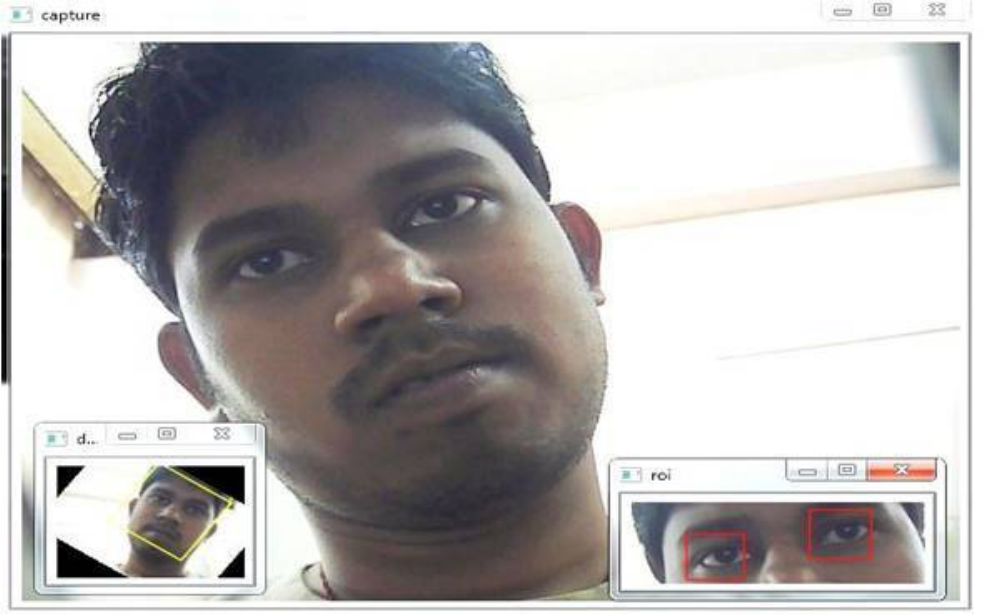}
\end{center}
   \caption{Tilted face detection using an affine transformation}
\label{fig:tilted_face}
\end{figure}

\subsection{Face tracking using Kalman Filter}

Detection of face using the modified Viola-Jones approach fails to detect face in some frames.  We have used 
Kalman Filter for tracking the face to avoid this issue. There are two advantages wit this tracking approach, 1) The predictions from kalman filter can be used to constrain the search space for face detection, 2) The prediciton from Kalman filter can be used as the tentative face location if the face detection stage fails. 
We have used a uniform velocity model for face tracking. In every frame the model is updated if the face detector returns the face location. In case the face detection fails, the predicted location from the Kalman filter is used as the tentative location of face.

The details of this approach can be found in our earlier works \cite{dasgupta2013board,dasgupta2013vision}.
